# Supplementary material for: Magpie: Alignment Data Synthesis from Scratch by Prompting Aligned LLMs with Nothing
Source: arXiv:2406.08464 source file (2024-10-07)
Supplement: Supplementary file 1 [file appendix01-extension.tex]

\section{\dataname{} Extension}
\label{appendix: magpie extension}

In this section, we explore the extension of \dataname{}. We first outline the process for constructing a multi-turn dataset (\dataname-MT). We then discuss methods for controlling instruction tasks using \dataname{}. Finally, we will briefly discuss how to develop a preference optimization dataset based on \dataname{}.

\subsection{Building Multi-Turn \dataname{}}

To construct a multi-turn dataset (\dataname-MT), we initially follow Steps 1 and 2 to generate the first turn of instruction and response. For subsequent turns, we append the pre-query template to the end of the full prompt from the previous round of communication. 
We have observed that the model may occasionally forget its role as the user, especially for the 8B model. To mitigate this, we employ a system prompt designed to control the behavior of the LLM and reinforce its awareness of the multi-round conversation context. The full prompt for building the instructions of \dataname-MT can be found in Figure \ref{fig: generating mt prompt} in Appendix \ref{appendix: prompt template}. We follow the procedure described in Step 2 of Section \ref{sec: method} to generate responses and yield the multi-turn instruction dataset.

\subsection{Control Instruction Tasks of \dataname{}}
In some scenarios, users may wish to fine-tune large language models (LLMs) using domain-specific instruction data, such as code or mathematical content, to enhance performance within specific domains. In this section, we introduce a lightweight and effective method to control the task category of generated instructions. Our approach involves guiding LLMs through the system prompt by specifying that it is a chatbot tailored for a particular domain and outlining the types of user queries it might encounter. We provide an example of a system prompt designed to control the generation of math-related instructions, as illustrated in Figure \ref{fig: control generation topic} within Appendix \ref{appendix: prompt template}.

\subsection{Building Preference Optimization Dataset with \dataname{}}

\dataname{} can be readily adapted to create preference datasets by integrating responses generated by the instruct model with those from the base model. Specifically, utilizing the reward difference outlined in Section \ref{sec:analysis}, a preference dataset can be assembled by designating the response from the instruct model as the preferred response, and the response from the base model as the less preferred one, provided that $r^*-r_{base} > 0$. We will soon open-source \dataname{}-PO, a preference optimization dataset to further align LLMs with human preferences.
